# Supplementary material for: Observation of non-Fermi liquid physics in a quantum critical metal via quantum loop topography
Source: arXiv:2007.07898 ancillary file (2020-07-15)
Supplement: Supplementary file 1 [file supplementary_materials.pdf]

# Supplementary Materials

George (Trey) Driskell<sup>1</sup>, Samuel Lederer<sup>1</sup>, Carsten Bauer<sup>2</sup>, Simon Trebst<sup>2</sup>, and Eun-Ah Kim<sup>1\*</sup>

<sup>1</sup>*Department of Physics, Cornell University, Ithaca, New York 14853, USA and*

<sup>2</sup>*Institute for Theoretical Physics, University of Cologne, 50937 Cologne, Germany*

(Dated: July 15, 2020)

## I. METHODS

### A. Classification metric and interpolation

The trained neural network outputs a number between 0 and 1 for each Monte Carlo sample (one Green function snapshot). The classification metric used in the paper consists of a numerical average of the neural network output for 800 such samples for the SDW model and 1600 samples for the nematic model. The color plots are produced using bilinear interpolation between the data points shown in Figure 1. The points are spaced closely in the horizontal direction (quantum tuning parameter) but are more distant in the vertical (temperature) direction.

### B. Training Details

The network was trained using stochastic gradient descent and standard practices of batch normalization following the hidden layer and  $L_2$  weight regularization to avoid overfitting. Batch normalization normalizes the hidden layer outputs during training by subtracting the mean and dividing by the standard deviation of the batch before the final layer.  $L_2$  weight regularization adds a term to the cost function proportional to the sum of the square of the neuron weight vectors. We found these augmentations to the training process insignificantly impacted the output phase diagram. The learning rate used during training was  $10^{-3}$ , and we employed early stopping to determine when the training of the neural network had plateaued. Varying the initial learning rate by a factor of 10 and dynamically reducing the learning rate based on the validation loss at each epoch both produced insignificantly different outputs.

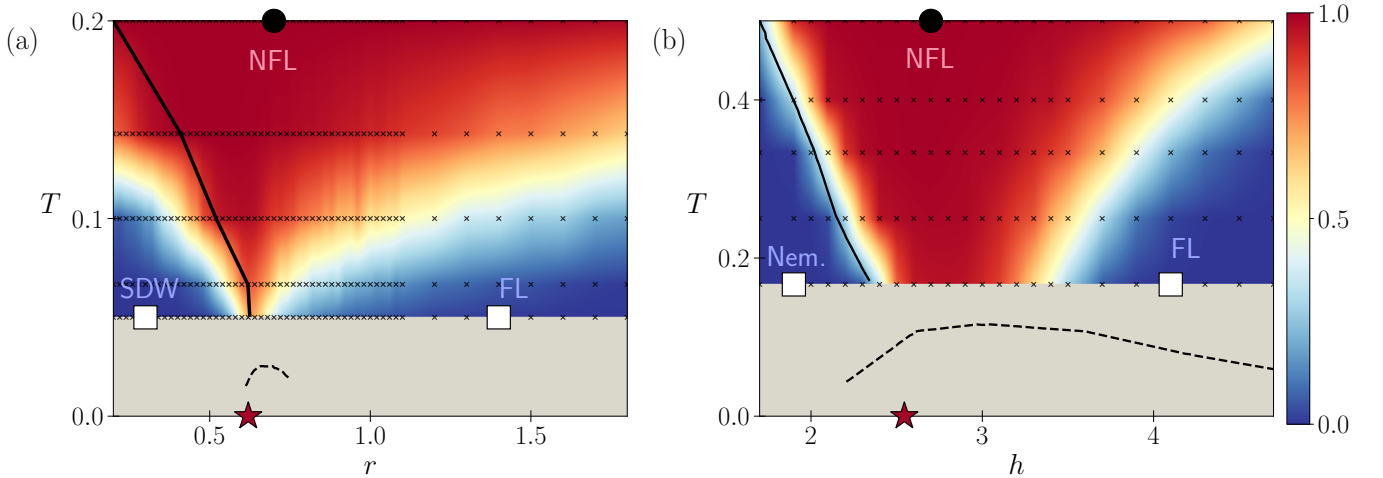

FIG. 1. **Data interpolation for both SDW and nematic models.** Both panels show the corresponding plots from Figure (1) in the main text with the data points overlaid as black x markers. In order to make the color plots, a bilinear spline is used to interpolate the values in between the available data points.

\* eun-ah.kim@cornell.edu

## II. ROBUSTNESS OF CLASSIFICATION FOR SDW MODEL

The network trained on QLT data yields predictions robust to substantial changes in the choice of training points for all three tasks. Figure 2 shows the robustness of the network's identification of the non-Fermi liquid regime: The phase diagram shows only modest quantitative changes when the non-Fermi liquid training point is moved closer to or further from the ordered phase (panels b and c), and similarly when the disordered Fermi liquid training point is moved (panels d and e). Figure 3 shows the robustness of the network's identification of the SDW phase: the phase diagram is essentially identical for several different choices of the training point for the disordered phase. Figure 4 shows the robustness of the network's identification of the disordered Fermi liquid regime to changes of the position of the training points for both the non-Fermi liquid (panels b and c) and Fermi liquid (panel d) regimes.

## III. ROBUSTNESS OF CLASSIFICATION FOR NEMATIC MODEL

The classification for the nematic model is also robust to changes in the training points, though somewhat less so than that of the SDW. Figure 5 shows the robustness of the network's identification of the non-Fermi liquid regime: The phase diagram shows only modest quantitative changes when the non-Fermi liquid training point is moved closer to or further from the ordered phase (panels b and c), and similarly when the disordered Fermi liquid training point is moved (panels d and e). Figure 6 shows the robustness of the network's identification of the nematic phase: the phase diagram is essentially identical for several different choices of the training point for the disordered phase. Figure 7 shows the robustness of the network's identification of the disordered Fermi liquid regime to changes of the position of the training points for both the non-Fermi liquid (panels b and c) and Fermi liquid (panel d) regimes.

Qualitative robustness notwithstanding, the network's predictions for the nematic model do have substantial dependence on the position of the disordered Fermi liquid training point. This is unlike the predictions for the SDW model, as can be seen by comparing figures 2 and 5. Linear preprocessing using only nearest neighbor Green's function data achieves superior stability in this respect, as can be seen in figure 8. Unlike the network in the main text, the network trained on nearest neighbor Green's functions shows the non-Fermi regime strongly narrowing as the temperature is lowered, regardless of the position of the disordered Fermi liquid training point. The lack of stability of the network involving QLT may reflect a quirk of the current operator in the nematic model: Because the nematic pseudospin  $\sigma_z$  lives on bonds, the current operator for a bond  $i, j$  will include a term proportional to  $\tau_{i,j}^z c_i^\dagger c_j$ . The absence of such terms in the QLT may rationalize some of the deficiencies of the QLT-trained network.

---

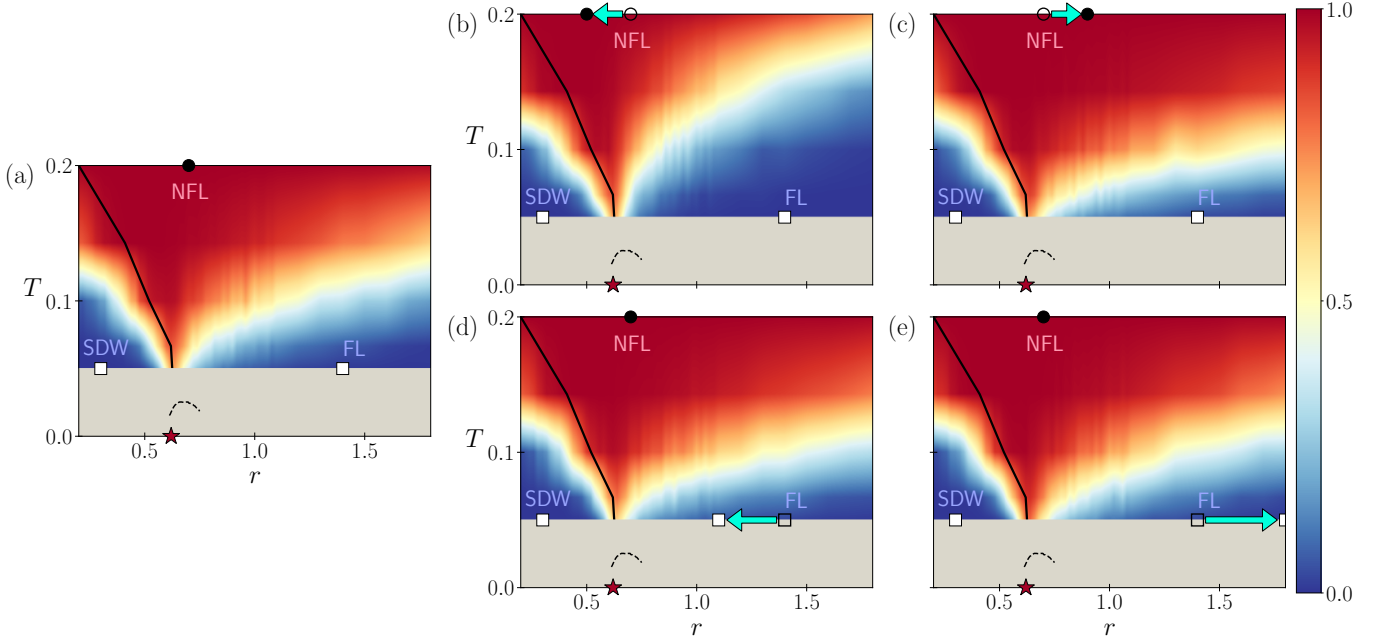

FIG. 2. **Robustness of three point non-Fermi liquid classification for the SDW model.** Panel (a) is the color plot in the main text. The remaining panels show that the classification varies only modestly when: (b) the non-Fermi liquid training point is moved closer to the ordered phase ( $r = 0.5$ ); (c) the non-Fermi liquid training point is moved further from the ordered phase ( $r = 0.9$ ); (d) the disordered Fermi liquid training point is moved closer to the QCP ( $r = 1.1$ ); (e) the disordered Fermi liquid training point is moved further from the QCP ( $r = 1.8$ ).

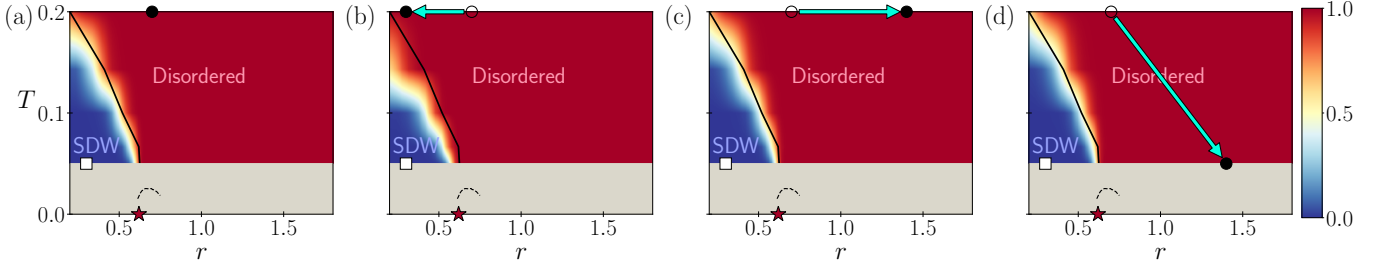

FIG. 3. **Robustness of phase classification for the SDW model.** Panel (a) is the color plot in the main text. The remaining panels show that the classification varies only modestly when: (b) the disordered phase training point is moved towards the ordered phase ( $r = 0.3$ ); (c) the disordered phase training point is moved away from the ordered phase ( $r = 1.4$ ); and (d) the disordered phase training point is moved to lower temperature and away from the ordered phase ( $r = 1.4, T = 0.05$ ).

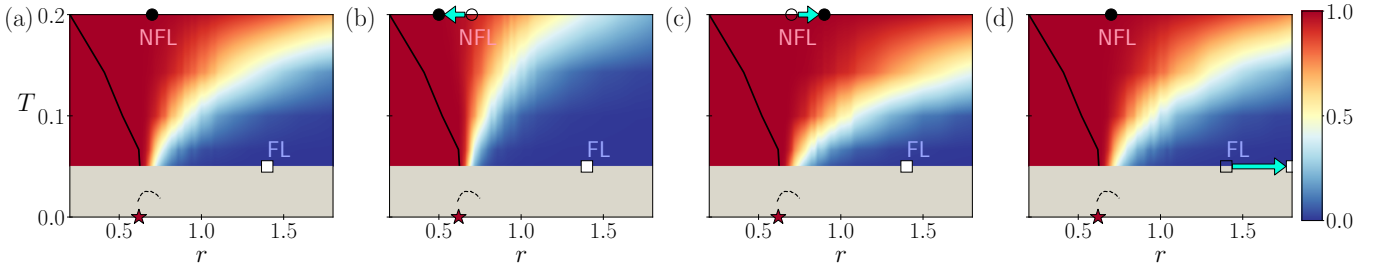

FIG. 4. **Robustness of the disordered Fermi liquid identification for the SDW model.** Panel (a) is the color plot in the main text. The remaining panels show that the classification varies only modestly when: (b) the non-Fermi liquid training point is moved towards the ordered phase ( $r = 0.5$ ); (c) the non-Fermi liquid training point is moved away from the ordered phase ( $r = 0.9$ ); and (d) the disordered Fermi liquid training point is moved further from the QCP ( $r = 1.8$ ).

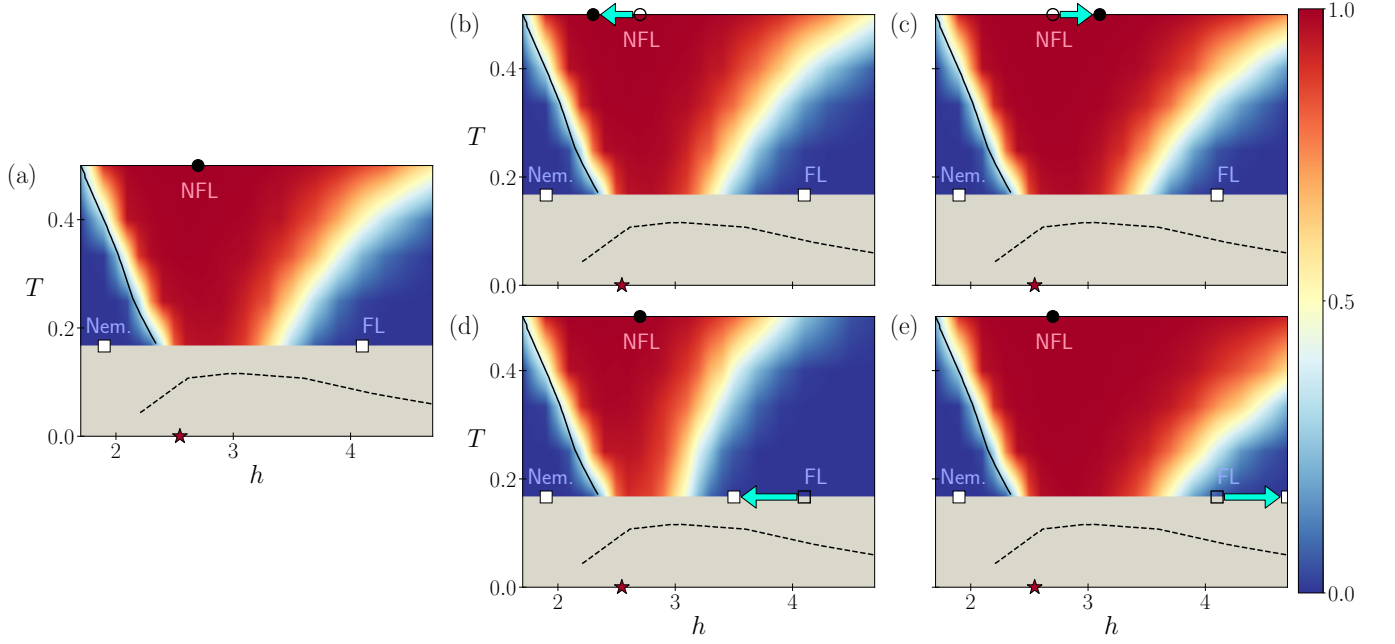

FIG. 5. **Robustness of three point classification for the nematic model.** Panel (a) is the color plot in the main text: the nematic ordered training point is located at  $h = 1.9, T = 0.167$ , the non-Fermi liquid training point at  $h = 2.7, T = 0.5$ , and the disordered Fermi liquid training point at  $h = 4.1, T = 0.167$ . Panels (b) and (c) move the non-Fermi liquid training point to  $h = 2.3$  and  $h = 3.1$  respectively at the same temperature. Panels (d) and (e) move the disordered Fermi liquid training point to  $h = 3.5$  and  $h = 4.7$  respectively at the same temperature.

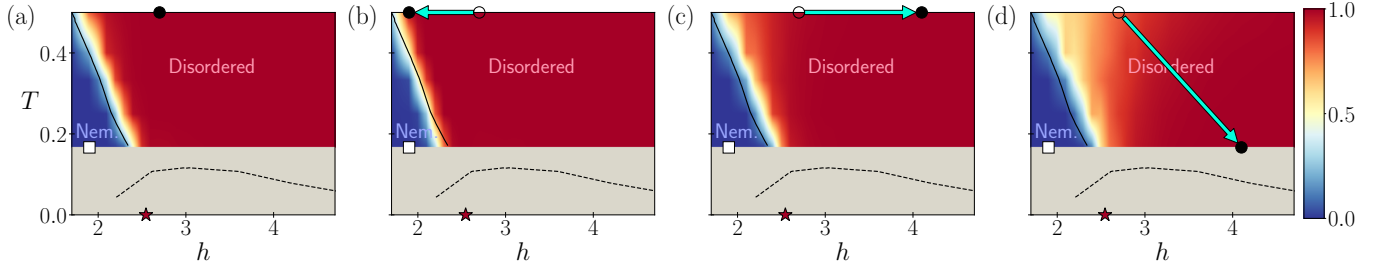

FIG. 6. **Robustness of phase classification for the nematic model.** Panel (a) is the color plot in the main text. The remaining panels show that the classification varies only modestly when: (b) the disordered phase training point is moved towards the ordered phase ( $h = 1.9$ ); (c) the disordered phase training point is moved away from the ordered phase ( $h = 4.1$ ); and (d) the disordered phase training point is moved to lower temperature and away from the ordered phase ( $h = 4.1, T = 0.167$ ).

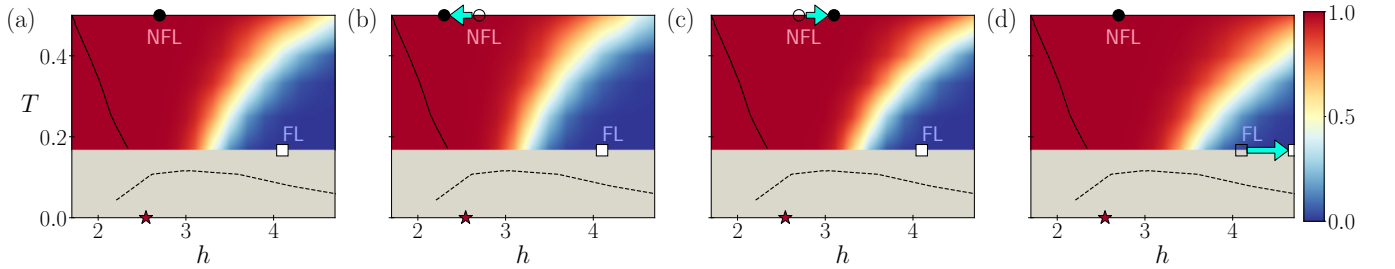

FIG. 7. **Robustness of disordered Fermi liquid identification for the nematic model.** Panel (a) is the color plot in the main text. The remaining panels show that the classification varies only modestly when: (b) the non-Fermi liquid training point is moved towards the ordered phase ( $h = 2.3$ ); (c) the non-Fermi liquid training point is moved away from the ordered phase ( $h = 3.1$ ); and (d) the disordered Fermi liquid training point is moved further from the QCP ( $h = 4.1$ ).

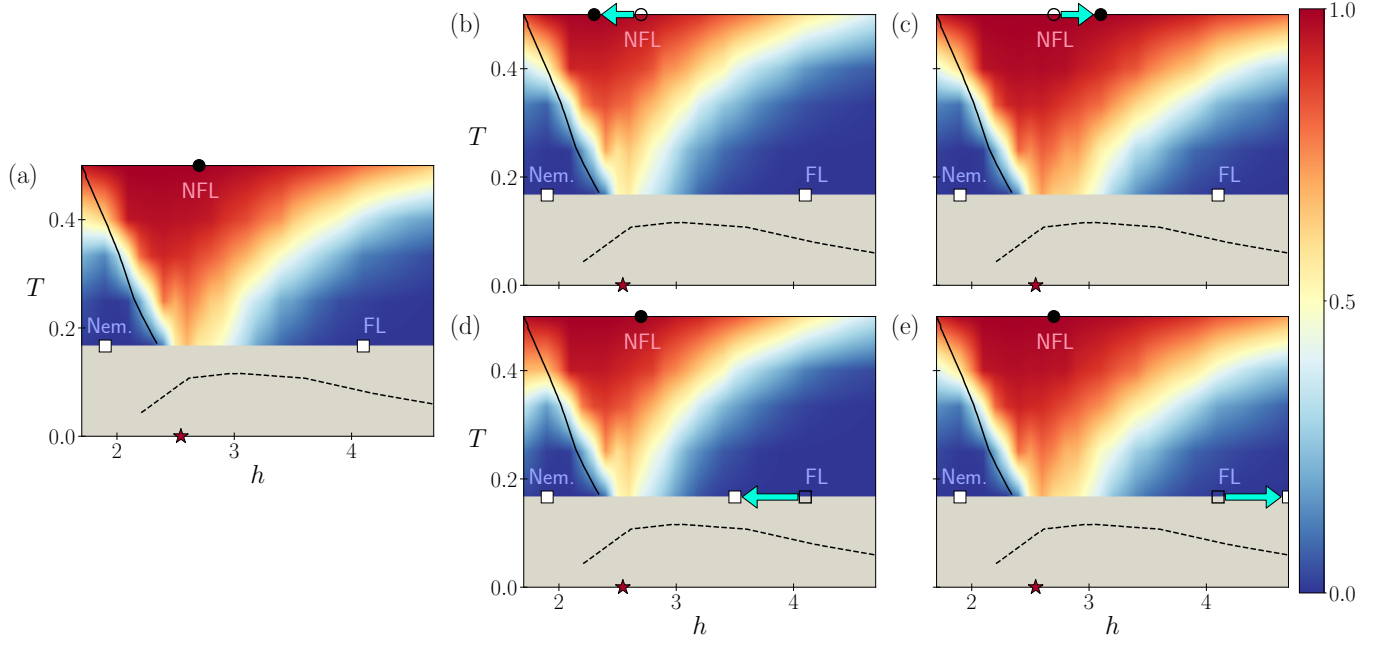

FIG. 8. **Three point non-Fermi liquid classification for the nematic model using only nearest neighbor Green's function data.** Panel (a) is the equivalent of the color plot in the main text. Panels (b) and (c) show that the classification varies only modestly when the non-Fermi liquid training point is moved towards ( $h = 2.3$ ) and away from ( $h = 3.1$ ) the ordered phase, respectively. Panels (d) and (e) show that the classification is qualitatively similar when the disordered Fermi liquid training point is moved towards ( $h = 3.5$ ) and away from ( $h = 4.7$ ) the QCP.
